# Supplementary material for: Asymmetric metasurfaces with high-$Q$ resonances governed by bound states in the continuum
Source: arXiv:1809.00330 ancillary file (2018-09-02)
Supplement: Supplementary file 1 [file supplemental_v3.pdf]

# Supplemental Material:
# Asymmetric metasurfaces with high-$Q$ resonances governed by bound states in the continuum

Kirill Koshelev[1,2], Sergey Lepeshov[2], Mingkai Liu[1], Andrey Bogdanov[2], and Yuri Kivshar[1,2]
[1]*Nonlinear Physics Centre, Australian National University, Canberra ACT 2601, Australia and*
[2]*ITMO University, St. Petersburg 197101, Russia*

In the Supplemental Material we (i) derive rigorously the transmission coefficient of a periodic photonic structure in the form of the classical Fano formula with explicit expressions for the Fano parameters, (ii) derive Eq. (2) of the main text, (iii) derive Eq. (3) of the main text, (iv) provide details on the eigenmode and reflection spectra dependence on the asymmetry parameter for designs of a metasurface with broken-symmetry meta-atoms shown in Figs.1(b-f) of the manuscript, (v) compare the results of the analytical approach shown in Fig. 4 with direct numerical simulations with realistic dispersion of silicon and (vi) calculate the BIC topological charge.

## S1. THE FANO FORMULA FOR THE TRANSMISSION COEFFICIENT OF PERIODIC STRUCTURES

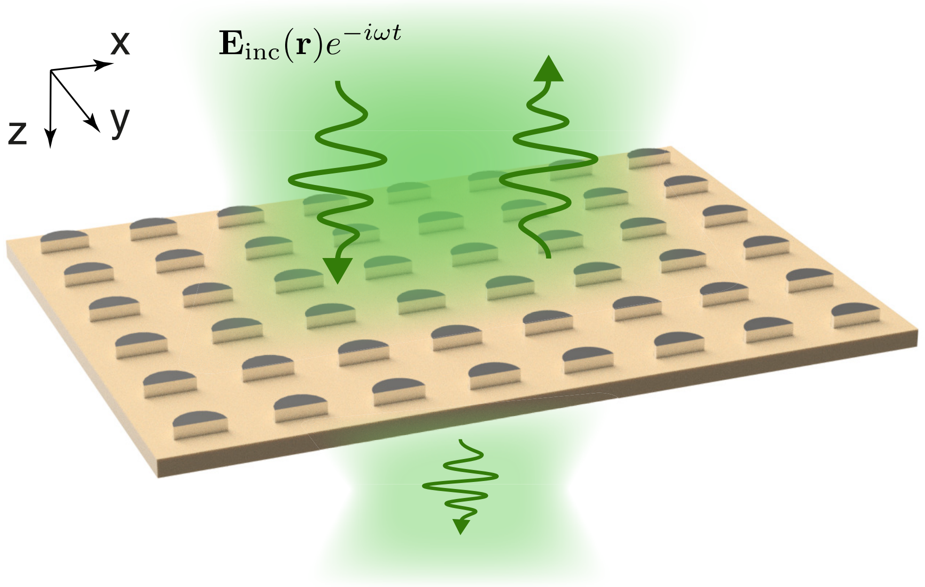


FIG. S1: Artistic view of light scattering by a metasurface.

We study the transmission amplitude $t$ of a periodic photonic structure made of material defined by the isotropic dielectric permittivity $\varepsilon(\omega,\mathbf{r})$, which is placed into the isotropic medium with permittivity 1. We assume normal incidence of a linearly x-polarized plane wave $\mathbf{E}_{\rm inc} = \mathbf{e}_x E_0 \exp{(ikz)}$ from the top of the structure (see Fig. S1) with real amplitude $E_0$.

The scattered field $\mathbf{E}_{\rm sc} = \mathbf{E} - \mathbf{E}_{\rm inc}$ satisfies the Lippmann-Schwinger equation [1]

$$\mathbf{E}_{\rm sc}(\mathbf{r}) = -k^2 \int d\mathbf{r}^{'} \, [\varepsilon(k,\mathbf{r}^{'})-1]\hat{\mathbf{G}}_0(k,\mathbf{r},\mathbf{r}^{'}) \cdot \left[\mathbf{E}_{\rm inc}(k,\mathbf{r}^{'}) + \mathbf{E}_{\rm sc}(\mathbf{r}^{'})\right], \tag{1}$$

where $k = \omega/c$, $\mathbf{E}$ is the total electric field, and $\hat{\mathbf{G}}_0$ is the free space dyadic Green's function (GF), satisfying the periodic boundary conditions. The scattered field in the integrand of Eq. (1) can be expressed in terms of the dyadic GF $\hat{\mathbf{G}}$ of the photonic structure

$$\mathbf{E}_{\rm sc}(\mathbf{r}^{'}) = -k^2 \int d\mathbf{r}^{''} \, [\varepsilon(k,\mathbf{r}^{''})-1]\hat{\mathbf{G}}(k,\mathbf{r}^{'},\mathbf{r}^{''}) \cdot \mathbf{E}_{\rm inc}(k,\mathbf{r}^{''}). \tag{2}$$

We focus on the case of periodic structures, which represent a rectangular array in x-y plane. The diagonal elements of $\hat{\mathbf{G}}_0$

can be calculated explicitly [2]

$$\left[\hat{G}_0(k,\mathbf{r},\mathbf{r}^{'})\right]_{xx,(yy)}=-\frac{i}{2k^2S_0}\sum_{\mathbf{L}}^{\infty}\frac{k^2-L^2_{x,(y)}}{\sqrt{k^2-\mathbf{L}^2}}\exp\left[-i\mathbf{L}(\mathbf{r}_{\|}-\mathbf{r}_{\|}^{'})+i|z-z^{'}|\sqrt{k^2-\mathbf{L}^2}\right], \tag{3}$$

where $S_0$ is the area of a unit cell of the periodic structure, $\mathbf{r}_{\|}=(x,y)$ is the in-plane position vector and $\mathbf{L}$ is the reciprocal lattice vector.

We consider periodic structures with sub-diffraction periods in both directions, thus all terms in Eq. (3) with $\mathbf{L}\neq 0$ are evanescent because $\sqrt{k^2-\mathbf{L}}$ is purely imaginary. To obtain the transmission we need the far-field expressions for the scattered field, so we leave the term with $\mathbf{L}=0$ only and Eq. (3) transforms into

$$\left[\hat{G}_0(k,\mathbf{r},\mathbf{r}^{'})\right]_{xx}=\left[\hat{G}_0(k,\mathbf{r},\mathbf{r}^{'})\right]_{yy}=-\frac{i}{2kS_0}e^{ik|z-z^{'}|}. \tag{4}$$

Within this approximation the far field expressions for the off-diagonal elements of the GF are equal to zero [2]

$$[\hat{G}_0]_{xy}=[\hat{G}_0]_{yx}=0 \tag{5}$$

The dyadic GF $\hat{\mathbf{G}}$ can be formally expressed through $\hat{\mathbf{G}}_0$ and the perturbation operator $\hat{W}$ which transforms free space into the photonic structure

$$\hat{\mathbf{G}}=\hat{\mathbf{G}}_0\left(1-\hat{W}\hat{\mathbf{G}}_0\right)^{-1}. \tag{6}$$

The operator $\hat{W}$ is a scalar, thus the combination of Eq. (5) and Eq. (6) provides that the off-diagonal elements of $\hat{\mathbf{G}}$ are also equal to zero in far-field. Since, we consider the x-polarized incident field, the scattered field is also x-polarized in far-field $\mathbf{E}_{\rm sc}=\mathbf{e}_x E_{\rm sc}$. Finally, by substituting Eq. (2) into Eq. (1) and projecting it to the x-axis we get

$$E_{\rm sc}(\mathbf{r})=-k^2E_0\int d\mathbf{r}^{'}\,[\varepsilon(k,\mathbf{r}^{'})-1]\left[\hat{G}_0(k,\mathbf{r},\mathbf{r}^{'})\right]_{xx}\left\{e^{ikz^{'}}-k^2\int d\mathbf{r}^{''}\,[\varepsilon(k,\mathbf{r}^{''})-1]\left[\hat{G}(k,\mathbf{r}^{'},\mathbf{r}^{''})\right]_{xx}e^{ikz^{''}}\right\}, \tag{7}$$

The key idea of our analysis which allows for rigorous treatment of the transmission coefficient is the explicit expansion of the GF $\hat{\mathbf{G}}$ over the eigenmodes (the resonant states) of the photonic structure $\mathbf{E}_j$ because they form the complete orthonormal basis inside the regions with material $\varepsilon(\omega,\mathbf{r}^{'})\neq 1$ [3]

$$\hat{\mathbf{G}}(k,\mathbf{r},\mathbf{r}^{'})=\sum_j\frac{\mathbf{E}_j(\mathbf{r})\mathbf{E}_j(\mathbf{r}^{'})}{2k(k-k_j)}+\Delta\hat{\mathbf{G}}(k,\mathbf{r},\mathbf{r}^{'}). \tag{8}$$

Here $j$ is the index of a resonant state, $\mathbf{E}_j(\mathbf{r})$ and $k_j=\omega_j/c$ is the electric field and and frequency of the eigenstate, respectively, and $\Delta\hat{\mathbf{G}}$ is the contribution of the Rayleigh anomalies, which can be expressed in terms of the resonant states lying in the cuts of the complex plane and can be calculated numerically with high precision [3].

The complex transmission amplitude $t$ can be expressed as

$$E_{\rm sc}(z\to\infty)=(t-1)E_0\exp{(ikz)}. \tag{9}$$

Using the expressions for the free-space GF [see Eq. (4)] and the photonic structure GF [see Eq. (8)] we can find $t$ explicitly

$$\begin{aligned}t(k)=1+\Delta t(k)+\frac{ik}{2S_0}[\varepsilon(k)-1]V_0-\\-\frac{ik^2}{4S_0}\sum_j\frac{\left(\int d\mathbf{r}^{'}[\varepsilon(k,\mathbf{r}^{'})-1]E_{j,x}(\mathbf{r}^{'})e^{-ikz^{'}}\right)\left(\int d\mathbf{r}^{''}[\varepsilon(k,\mathbf{r}^{''})-1]E_{j,x}(\mathbf{r}^{''})e^{ikz^{''}}\right)}{k-k_j},\end{aligned} \tag{10}$$

$$\Delta t(k)=-\frac{ik^3}{2S_0}\int d\mathbf{r}^{'}\,[\varepsilon(k,\mathbf{r}^{'})-1]e^{-ikz^{'}}\int d\mathbf{r}^{''}\,[\varepsilon(k,\mathbf{r}^{''})-1]e^{ikz^{''}}\left[\Delta\hat{G}(k,\mathbf{r}^{'},\mathbf{r}^{''})\right]_{xx}. \tag{11}$$

Here $V_0$ is the volume of a single meta-atom.

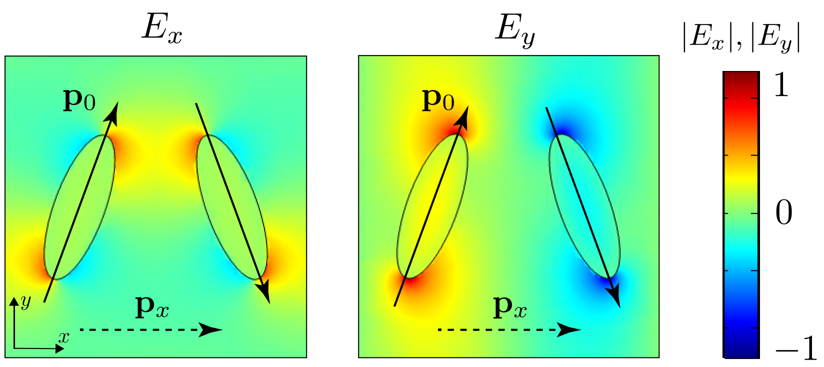


FIG. S2: Electric field component patterns for the quasi-BIC analyzed in the main text. Arrows show the dipole moments: $\mathbf{p}_0$ is the dipole moment of a single bar, $\mathbf{p}_x$ is the net dipole moment of the unit cell.

Next, we introduce coupling amplitude

$$D_{j,x}(k) = -\frac{k}{\sqrt{2S_0}} \int d\mathbf{r}^{'} [\varepsilon(k, \mathbf{r}^{'}) - 1] E_{j,x}(\mathbf{r}^{'}) e^{ikz^{'}}. \tag{12}$$

Each resonant state can be classified with respect to the up-down mirror symmetry $E_{j,x}(-z) = (-1)^p E_{j,x}(z)$, where $p = 0, 1$ corresponds to an even or an odd state, respectively. Thus, Eq. (10) can be written as

$$t(k) = 1 + \Delta t(k) + \frac{ik}{2S_0}[\varepsilon(k) - 1]V_0 - i \sum_j \frac{(-1)^p \left[D_{j,x}(k)\right]^2}{2(k - k_j)}, \tag{13}$$

We focus on the frequency region in the vicinity of the eigenfrequency $ck_{j_0} = \omega_0 - i\gamma/2$ of the particular resonant state with index $j_0$ and parity $p_0$, where $\omega_0$ is the resonant frequency and $\gamma$ is the mode inverse radiation lifetime. Then, $t$ can be expressed as

$$t(k) = B(k) - i\frac{A(k)}{\Omega + i}, \tag{14}$$

where the coefficients are determined below

$$A(k) = \frac{(-1)^{p_0} \left[D_{j_0,x}(k)\right]^2}{\gamma/c}, \tag{15a}$$

$$B(k) = 1 + \Delta t(k) + \frac{ik}{2S_0}[\varepsilon(k) - 1]V_0 - i \sum_{j \neq j_0} \frac{(-1)^p \left[D_{j,x}(k)\right]^2}{2(k - k_j)}, \tag{15b}$$

$$\Omega = \frac{2(\omega - \omega_0)}{\gamma} \tag{15c}$$

By straightforward but quite cumbersome rearrangements of terms of Eq. (14) the transmission coefficient can be written in the form of the classical Fano formula

$$T(\omega) = \frac{T_0(\omega)}{1 + q^2(\omega)} \frac{[q(\omega) + \Omega]^2}{1 + \Omega^2} + T_{\rm bg}(\omega). \tag{16}$$

The parameters are

$$q(\omega) = \tan\psi, \tag{17a}$$

$$\psi(\omega) = \frac{1}{2}\cot^{-1}\left(\cot\Delta - \frac{|A|}{2|B|\sin\Delta}\right), \tag{17b}$$

$$\Delta(\omega) = \arg\left(AB^*\right), \tag{17c}$$

$$T_0(\omega) = |A|\left(|A|^2 - 4|A||B|\cos\Delta + 4|B|^2\right)^{1/2}, \tag{17d}$$

$$T_{\rm bg}(\omega) = |B|^2 - \frac{T_0}{1 + q^2}, \tag{17e}$$

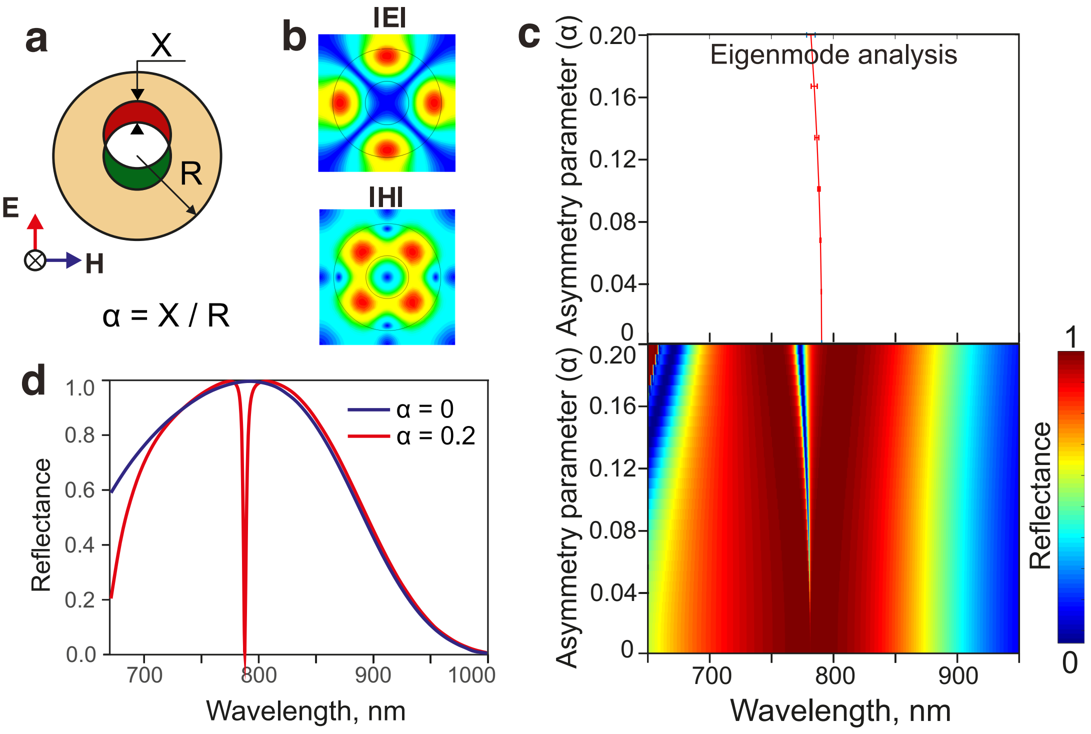


FIG. S3: (a) Design of the unit cell of a metasurface shown in Fig.1b of the manuscript. Parameters: a metasurface with the square lattice in free-space, the period is 380 nm, the outer radius is 150 nm, the inner radius is 60 nm, the height is 200 nm, the permittivity is 13.5. (b) Distribution of the electric and magnetic fields for the BIC. (c) Eigenmode spectra and reflectance with respect to pump wavelength and asymmetry parameter $\alpha$. Error bars show the magnitude of the mode inverse radiation lifetime. (d) Evolution of the reflectance vs. $\alpha$.

where $q$ is the Fano asymmetry parameter.

Here we use the first and the last assumption that for $\omega$ in the vicinity of $\omega_0$ the frequency dependence $\Delta(\omega)$, $q(\omega)$, $T_0(\omega)$ and $T_{\text{bg}}(\omega)$ is smooth and can be neglected. This assumption is valid when the neighboring resonances do not overlap with the resonant state of interest. It is worth mentioning that the same analysis can be applied to show that the reflection coefficient $R$ can be rigorously written in the form of the classical Fano formula.

We analyse the applicability of Eq. (16) for analysis of metasurfaces with symmetric meta-atoms which support true BICs. In this case the electric field component $E_{j_0,x}$ of a BIC is odd with respect to in-plane inversion symmetry $E_{j_0,x}(-x,-y) = -E_{j_0,x}(x,y)$, therefore, from Eq. (12) it follows that coupling amplitude $D_{j_0,x} = 0$. Thus, $A = 0$ and $\Delta$ becomes indefinite. Finally, Eqs. (17a-c) show that the Fano asymmetry parameter $q$ becomes ill-defined for a true BIC.

## S2. DERIVATION OF EQUATION (2)

We start with showing how a resonant state can be treated as an eigenmode of a closed resonator interacting with the radiation continuum. The derivation can be performed rigorously using the approach based on the Fano-Feshbach projection scheme [4]. However, here we apply another method based on the perturbation theory.

We study a periodic photonic structure, which represents an open electromagnetic resonator. Here, for the sake of simplicity, we consider the structure with the constant real-valued permittivity $\varepsilon(\mathbf{r})$ surrounded by the isotropic environment, however, the approach can be easily expanded to a more general case of a dispersive material with losses and a substrate. Also, we consider the sub-diffraction regime when the wavelength of interest is larger than both periods. We focus on the particular resonant state $\mathbf{E}_{\text{rs}}$. We enclose the resonator with two flat boundaries parallel to the structure surface, which are placed above and below the structure in the far field of the resonant state and are characterized by the normals $\mathbf{s} = \mathbf{e}_z$ and $\mathbf{s} = -\mathbf{e}_z$. While radiation losses are weak, the resonant state can be divided into sum

$$\mathbf{E}_{\text{rs}}(\mathbf{r}) = \mathbf{E}^{(0)}(\mathbf{r}) + \delta\mathbf{E}(\mathbf{r}), \tag{18}$$

where $\mathbf{E}^{(0)}(\mathbf{r})$ is the solution of Maxwell's equations in the space between two boundaries which satisfies the perfect magnetic

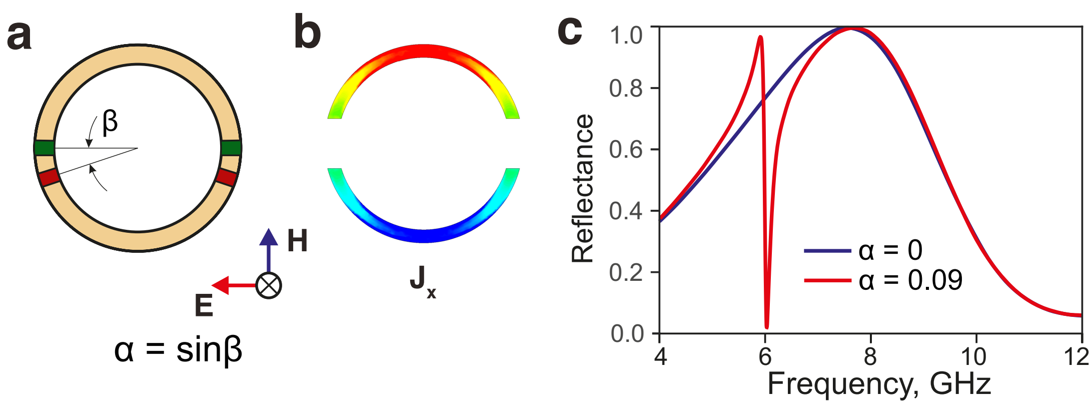


FIG. S4: (a) Design of the unit cell of a metasurface shown in Fig.1c of the manuscript. Parameters: a metasurface with the square lattice in free-space, the period is 15 mm, the inner radius is 5.2 mm, the ring thickness is 0.8 mm, the height is 35 $\mu$m, the distance between semi-rings is 3 mm, the material is copper. (b) Distribution of the current for the BIC. (c) Evolution of the reflectance vs. $\alpha$.

boundary conditions

$$\mathbf{s} \times \nabla \times \mathbf{E}^{(0)} = 0. \tag{19}$$

Since we study the modes with quality factor larger than 10, the term $\delta\mathbf{E}(\mathbf{r})$ is the perturbation of $\mathbf{E}^{(0)}(\mathbf{r})$.

The resonant state is normalised as [3]

$$1 = \int_V dV\, \varepsilon \mathbf{E}_{\rm rs} \cdot \mathbf{E}_{\rm rs} + \frac{c^2}{2\omega_{\rm rs}^2} S_0 \sum_{s=\pm 1} s \left( \mathbf{E}_{\rm rs} \cdot \frac{\partial^2 \mathbf{E}_{\rm rs}^{\rm (reg)}(\omega)}{\partial z \partial \omega}\bigg|_{\omega=\omega_{\rm rs}} - \frac{\partial \mathbf{E}_{\rm rs}}{\partial z} \cdot \frac{\partial \mathbf{E}_{\rm rs}^{\rm (reg)}(\omega)}{\partial \omega}\bigg|_{\omega=\omega_{\rm rs}} \right)\bigg|_{z\in S}, \tag{20}$$

where $S$ is the surface of the magnetic boundaries, $S_0$ is the surface area of a unit cell, the volume integration is performed between the boundaries and $\mathbf{E}_{\rm rs}^{\rm (reg)}$ is the analytical continuation of $\mathbf{E}_{\rm rs}$ to the whole $\omega$-plane. Here we used the fact $\mathbf{E}_{\rm rs}$ represents a plane wave at the boundaries since they lie in the far field of the resonant state and its frequency is below the diffraction limit.

The boundary conditions Eq. (19) imply that for $\mathbf{E}^{(0)}(\mathbf{r})$ the right term in Eq. (20) is zero and the normalization within the zero order of the perturbation theory is

$$1 = \int_V dV\, \varepsilon \mathbf{E}^{(0)} \cdot \mathbf{E}^{(0)}. \tag{21}$$

Here we choose $\mathbf{E}^{(0)}$ to be a real-valued function.

For each resonant state $\mathbf{E}_{\rm rs}$ with complex frequency $\omega_{\rm rs} = \omega_0 - i\gamma/2$ the another resonant state with frequency $-\omega_0 - i\gamma/2$ and field $\mathbf{E}_{\rm rs}^*$ must exist in the spectrum of an open system which is a direct consequence of Maxwell's equations. We can find the elegant formula for the inverse radiation lifetime $\gamma$ by exploiting the orthogonality condition between these complementary resonant states [3]

$$0 = [\omega_{\rm rs}^2 - (\omega_{\rm rs}^*)^2] \int_V dV\, \varepsilon \mathbf{E}_{\rm rs} \cdot \mathbf{E}_{\rm rs}^* - c^2 S_0 \sum_{s=\pm 1} s \left( \mathbf{E}_{\rm rs} \cdot \frac{\partial \mathbf{E}_{\rm rs}^*}{\partial z} - \mathbf{E}_{\rm rs}^* \cdot \frac{\partial \mathbf{E}_{\rm rs}}{\partial z} \right)\bigg|_{z\in S}. \tag{22}$$

Since the surface $S$ is located in the far field of the resonant state, we can use the relation $\partial \mathbf{E}_{\rm rs}/\partial z = is\omega_{\rm rs}/c\, \mathbf{E}_{\rm rs}$ and simplify Eq. (22) to the form

$$\frac{\gamma}{c} = \frac{S_0 \sum_{s=\pm 1} \left( |\mathbf{E}_{\rm rs}|^2 \right)\big|_{z\in S}}{\int_V dV\, \varepsilon |\mathbf{E}_{\rm rs}|^2}. \tag{23}$$

Within the first order perturbation theory (see Eq. (21)] Eq. (23) is reduced to

$$\frac{\gamma}{c} = S_0 \sum_{s=\pm 1} \left( |E_{{\rm rs},x}|^2 + |E_{{\rm rs},y}|^2 \right)\bigg|_{z\in S}. \tag{24}$$

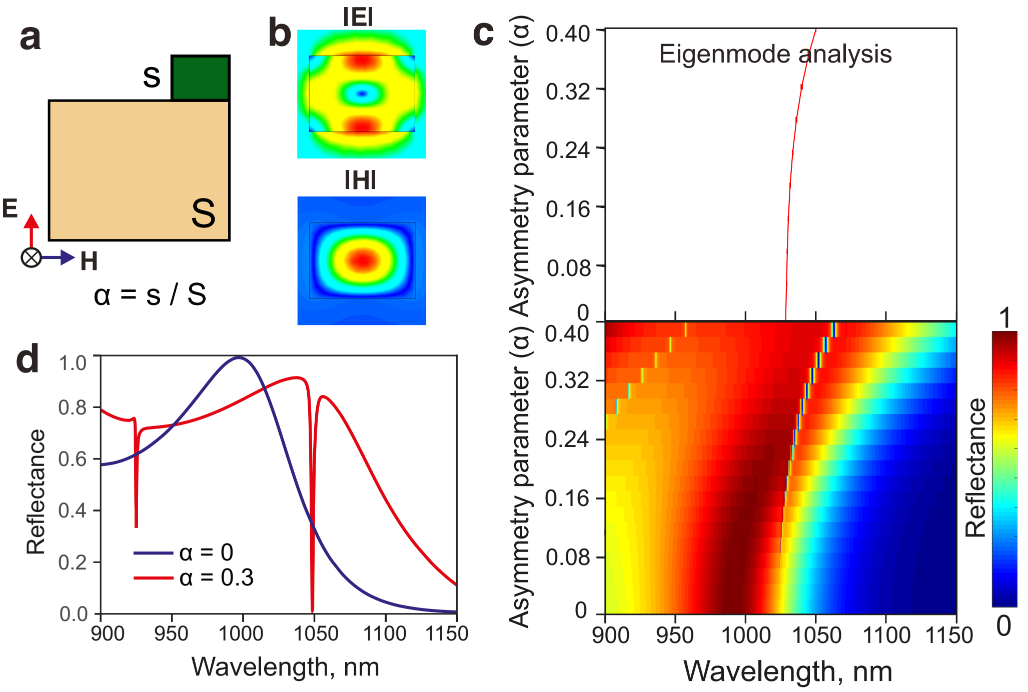


FIG. S5: (a) Design of the unit cell of a metasurface shown in Fig.1d of the manuscript. Parameters: a metasurface with the square lattice in free-space, the period is 550 nm, large bar size is 200 × 280 (nm×nm), the height is 250 nm, the permittivity is 13.5. (b) Distribution of the electric and magnetic fields for the BIC. (c) Eigenmode spectra and reflectance with respect to pump wavelength and asymmetry parameter $\alpha$. Error bars show the magnitude of the mode inverse radiation lifetime. (d) Evolution of the reflectance vs. $\alpha$.

To calculate the sum we apply the Lippmann-Schwinger equation to the resonant state

$$\mathbf{E}_{\rm rs}(\mathbf{r}) = -\frac{\omega_{\rm rs}^2}{c^2}\int d\mathbf{r}^{'}\ [\varepsilon(\omega_{\rm rs},\mathbf{r}^{'})-1]\hat{\mathbf{G}}_0(\omega_{\rm rs},\mathbf{r},\mathbf{r}^{'})\cdot\mathbf{E}_{\rm rs}(\mathbf{r}^{'}). \tag{25}$$

Using the perturbation theory it can be transformed to

$$\mathbf{E}_{\rm rs}(\mathbf{r}) = -\frac{\omega_0^2}{c^2}\int d\mathbf{r}^{'}\ [\varepsilon(\omega_0,\mathbf{r}^{'})-1]\hat{\mathbf{G}}_0(\omega_0,\mathbf{r},\mathbf{r}^{'})\cdot\mathbf{E}_{\rm rs}(\mathbf{r}^{'}). \tag{26}$$

In section S1 [see Eq.( 5)] we showed that off-diagonal elements of the free-space GF $\hat{\mathbf{G}}_0$ are equal to zero. Using the sub-diffraction limit and the far-field expressions for the diagonal elements [see Eq. (4)] we can express the components of $\mathbf{E}_{\rm rs}(\mathbf{r})$ at each boundary as

$$\left|E_{{\rm rs},x(y)}(z\to\infty)\right|^2 = \frac{\omega_0^2}{4S_0^2c^2}\left|\int d\mathbf{r}^{'}\ [\varepsilon(\omega_0,\mathbf{r}^{'})-1]E_{{\rm rs},x(y)}(\mathbf{r}^{'})e^{-ik_0z^{'}}\right|^2, \tag{27a}$$

$$\left|E_{{\rm rs},x(y)}(z\to-\infty)\right|^2 = \frac{\omega_0^2}{4S_0^2c^2}\left|\int d\mathbf{r}^{'}\ [\varepsilon(\omega_0,\mathbf{r}^{'})-1]E_{{\rm rs},x(y)}(\mathbf{r}^{'})e^{ik_0z^{'}}\right|^2. \tag{27b}$$

As it was mentioned in Section S1 the resonant state can be classified with respect to the up-down symmetry $E_x(-z) = (-1)^pE_x(z)$, thus we can equate Eq. (27a) and Eq. (27b). Now we substitute Eqs. (27a-b) into Eq. (24) and sum all terms. Then the mode inverse lifetime is

$$\frac{\gamma}{c} = |D_x|^2 + |D_y|^2. \tag{28}$$

Here the coupling amplitudes $D_i$ are the same as $D_{j,x}$ in Eq. (12) which can be explained by the reciprocity of the system

$$D_i = -\frac{\omega_0}{\sqrt{2S_0}c}\int d\mathbf{r}^{'}\ [\varepsilon(\omega_0,\mathbf{r}^{'})-1]E_{{\rm rs},i}(\mathbf{r}^{'})e^{ik_0z^{'}}, \qquad i=x,y. \tag{29}$$

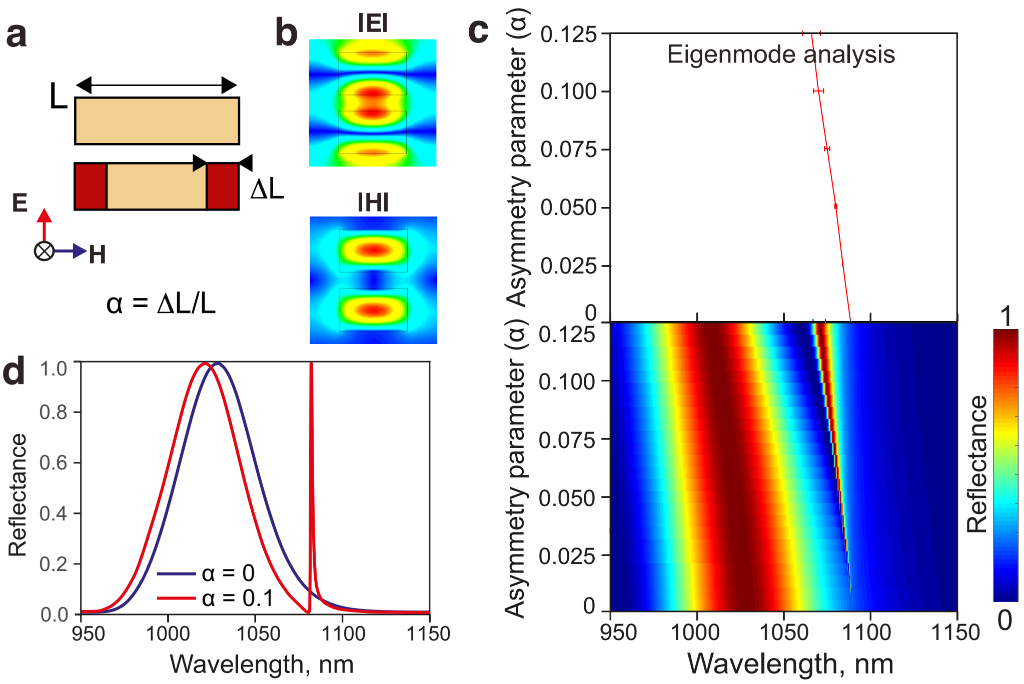


FIG. S6: (a) Design of the unit cell of a metasurface shown in Fig.1e of the manuscript. Parameters: a metasurface with the rectangular lattice in free-space, the period in x direction is 725 nm, the period in y direction is 530 nm, large bar size is 200 × 280 (nm×nm), the height is 250 nm, distance between bars is 75 nm, the permittivity is 13.5. (b) Distribution of the electric and magnetic fields for the BIC. (c) Eigenmode spectra and reflectance with respect to pump wavelength and asymmetry parameter $\alpha$. Error bars show the magnitude of the mode inverse radiation lifetime. (d) Evolution of the reflectance vs. $\alpha$.

A simplification of Eq. (29) can be achieved by expanding the function $e^{ik_0 z'}$ into the Taylor series. Thus, the coupling amplitudes $D_i$ can be found as

$$D_x = -\frac{k_0}{\sqrt{2S_0}}\left[p_x - \frac{m_y}{c} + \frac{ik_0}{6}Q_{zx}\right], \tag{30a}$$

$$D_y = -\frac{k_0}{\sqrt{2S_0}}\left[p_y + \frac{m_x}{c} + \frac{ik_0}{6}Q_{yz}\right], \tag{30b}$$

where $\mathbf{p}$, $\mathbf{m}$ and $\hat{\mathbf{Q}}$ are the electric dipole, magnetic dipole and electric quadrupole moments in the irreducible representations defined as in Ref. 5. Since the thickness of a metasurface is small compared to the period and we analyze the quasi-BIC which frequency is below the diffraction limit, the condition $k_0 z < 1$ is fulfilled inside the resonators, thus, higher order multipoles in Eqs. (30a-b) are not relevant.

## S3. DERIVATION OF EQUATION (3)

To derive Eq.(3) for the metasurface with tilted silicon bars we simplify Eq. (28) using the symmetry properties of the BIC and the quasi-BIC. When the bars are rotated, the unit cell symmetry with respect to $(x) \to (-x)$ mirror transformation remains conserved. Therefore, $E_{\mathrm{rs},x}$ and $E_{\mathrm{rs},y}$ can be classified as even and odd functions with respect to this symmetry. Importantly, x- and y-components of electric field always have different parity with respect to this symmetry. Numerical analysis shown in Fig.S2 demonstrates that $E_{\mathrm{rs},x}$ is even and $E_{\mathrm{rs},y}$ is odd. Therefore, from Eq. (29) it follows that $D_y = 0$ for the quasi-BIC supported by a metasurface with arbitrary angle $\theta$ of bar rotation. Next, terms $m_y$ and $Q_{zx}$ in Eq. (30a) are equal to zero because $E_{\mathrm{rs},x}(-z) = E_{\mathrm{rs},x}(z)$. After these simplifications Eq. (28) is transformed as follows

$$\frac{\gamma_{\mathrm{rad}}}{c} = \frac{k_0^2}{2S_0}\,|p_x|^2\,. \tag{31}$$

Each bar has a dipole moment $\mathbf{p}_0$ shown in Fig.S2. The y-components of $\mathbf{p}_0$ for two bars are opposite. For $\theta > 0$, $p_x$ is defined as the net dipole moment between two bars. For small angles $\mathbf{p}_0 = \mathbf{e}_y p_0$, where $p_0$ is evaluated for $\theta = 0°$. Thus, the

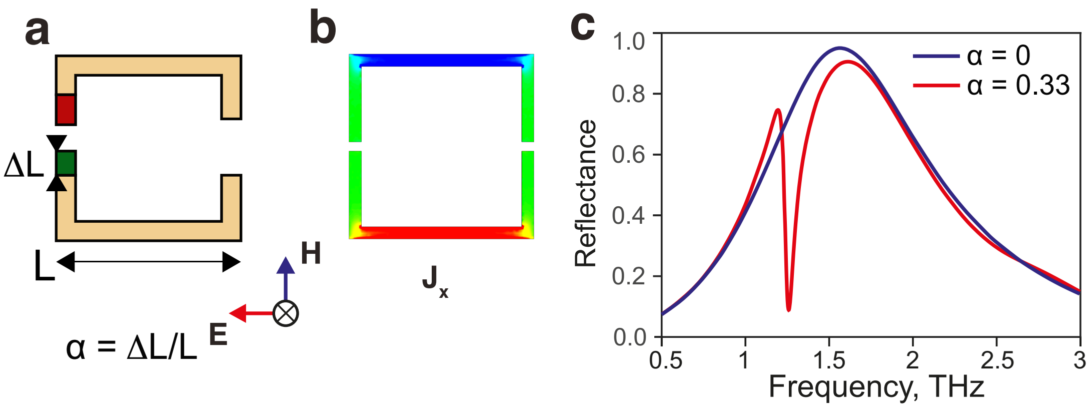


FIG. S7: (a) Design of the unit cell of a metasurface shown in Fig.1f of the manuscript. Parameters: a metasurface with the square lattice in free-space, the period is 75 $\mu$m, the large square side is 60 $\mu$m, the ring thickness is 4 $\mu$m, the height is 0.2 $\mu$m, distance between semi-rings is 3 $\mu$m, the material is aluminium, the conductance is $3.56 \times 10^7$ S/m. (b) Distribution of the current for the BIC. (c) Evolution of the reflectance vs. $\alpha$.

net dipole moment is

$$p_x = 2p_0 \sin\theta, \tag{32a}$$

$$p_0 = \int d\mathbf{r}\, [\varepsilon(\omega_0, \mathbf{r}) - 1] E_{\text{rs},y}(\theta = 0^\circ, \mathbf{r}). \tag{32b}$$

Finally, the radiative quality factor $Q_{\text{rad}} = \omega_0/\gamma_{\text{rad}}$ can be found as

$$Q_{\text{rad}} = \frac{S_0}{2k_0} |p_0|^{-2} (\sin\theta)^{-2}. \tag{33}$$

Therefore, we arrive at Eq.(3) of the manuscript with parameter $Q_0$ defined as

$$Q_0 = \frac{S_0}{2k_0} \left| \int d\mathbf{r}\, [\varepsilon(\omega_0, \mathbf{r}) - 1] E_{\text{rs},y}(\theta = 0^\circ, \mathbf{r}) \right|^{-2}. \tag{34}$$

Importantly, here $\mathbf{E}_{\text{rs}}$ is normalized according to Eq. (21).

Finally, we derive Eq. (3) for a general type of metasurfaces with asymmetric meta-atoms using the second order perturbation theory for non-Hermitian open systems similarly to the analysis in Ref. 3. We consider that a metasurface with a symmetric unit cell is characterized by a basis of resonant states with electric fields $\mathbf{E}_n^{(0)}$ and complex frequencies $\omega_n^{(0)}$. We introduce a perturbation of the unit cell $\hat{V}(\mathbf{r}) = \Delta\varepsilon(\mathbf{r})$ which breaks the in-plane inversion symmetry; examples of perturbation profiles are shown in Fig. 3(b) of the text. The resonant states electric field $\mathbf{E}_n$ of the perturbed metasurface can be found via the expansion

$$\mathbf{E}_n = \sum_n b_m^n \mathbf{E}_m^{(0)}. \tag{35}$$

The coefficients $b_m^n$ and new eigenfrequencies $\omega_n$ can be found using the resonant-state expansion [3]

$$\frac{1}{\omega_n^{(0)}} b_n^n + \sum_m \frac{1}{2} \frac{V_{nm}}{\left(\omega_n^{(0)}\right)^{\frac{1}{2}} \left(\omega_m^{(0)}\right)^{\frac{1}{2}}} b_m^n = \frac{1}{\omega_n} b_n^n, \tag{36a}$$

$$V_{nm} = \int d\mathbf{r}\, \Delta\varepsilon(\mathbf{r}) \mathbf{E}_n^{(0)} \cdot \mathbf{E}_m^{(0)}. \tag{36b}$$

Considering $\hat{V}$ as a small perturbation and using the second-order perturbation theory for non-Hermitian systems we find new eigenfrequencies as

$$\omega_n = \omega_n^{(0)} \left( 1 - \frac{1}{2} V_{nn} + \frac{1}{4} V_{nn}^2 + \sum_m \frac{1}{4} \frac{\omega_n^{(0)} V_{nm}^2}{\omega_n^{(0)} - \omega_m^{(0)}} \right). \tag{37}$$

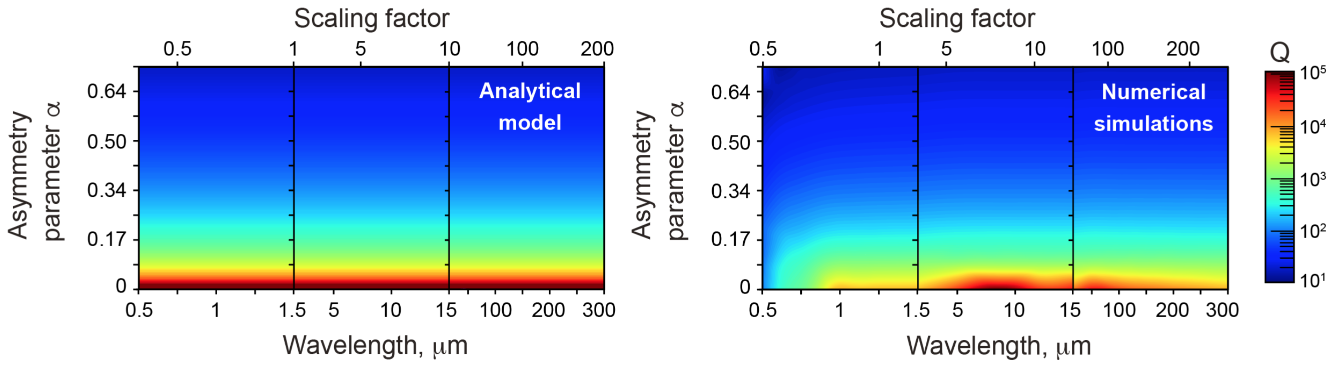


FIG. S8: Map of operating wavelengths and quality factors available for silicon metasurfaces with tilted-bar pairs by controlling the angle between bars ($\alpha = \sin\theta$) and the geometrical parameter. Left panel: analytical results based on Eq. (3) of the main text. Right panel: direct numerical simulations with realistic dispersion of silicon shown in lower. Geometric scaling factor is shown in the upper horizontal axis.

We focus on a BIC with the real frequency $\omega_{n_0}^{(0)}$ which transforms into a quasi-BIC with the complex frequency $\omega_{n_0}$. Since the electric field of the BIC can be chosen as a real-valued function, the matrix element $V_{n_0n_0}$ is real. Thus, the imaginary part of $\omega_{n_0}$ is contributed by the last term of Eq. 37 only. Therefore, the quasi-BIC radiative Q factor can be found as

$$Q_{\rm rad}^{-1} = \frac{\omega_{n_0}^{(0)}}{2}{\rm Im}\left(\sum_m \frac{V_{n_0m}^2}{\omega_m^{(0)} - \omega_{n_0}^{(0)}}\right). \tag{38}$$

Remarkably, Eq. 38 shows that the BIC can be destroyed only due to coupling to leaky resonant states.

Finally, for small perturbations $V_{n_0m}$ is proportional to the asymmetry parameter $\alpha$. Therefore, we arrive at Eq. (3) of the main text

$$Q_{\rm rad} \propto \alpha^{-2}. \tag{39}$$

## S4. EIGENMODE SPECTRA AND REFLECTANCE FOR OTHER DESIGNS OF METASURFACES

In this section provide details on eigenmode spectra and reflectance dependence on the asymmetry parameter for designs of a metasurface with broken-symmetry meta-atoms shown in Fig. 1(b-f) of the manuscript. The results with descriptions are shown in Figs. S3-S7.

## S5. COMPARISON OF FIG. 4 WITH NUMERICAL SIMULATIONS WITH REALISTIC DISPERSION OF SILICON

In this section we compare the results of the analytical approach shown in Fig. 4 of the main text with direct numerical simulations using the realistic dispersion of silicon. We verify the applicability of the proposed analytical approach by three-dimensional electromagnetic simulations with the silicon dispersion by exploiting the finite-element method in COMSOL, and the results are shown in Fig. S8. Both approaches agree well, thus justifying the validity of the analytical scaling method.

## S6. TOLOPOLOGICAL CHARGE OF BIC

In this section we calculate the topological charge of the BIC supported by a metasurface with tilted silicon-bar pairs analysed in in Fig.2 of the main text. Here we follow the procedure described in Ref. [6]. The topological charge $q_{\rm top}$ carried by a BIC is defined as

$$q_{\rm top} = \frac{1}{2\pi}\oint d\mathbf{k}\cdot\nabla_{\mathbf{k}}\varphi(\mathbf{k}), \tag{40}$$

where the integration domain is a closed simple path in $\mathbf{k}$-space that goes around the BIC in the counterclockwise direction. We define the angle of polarization vector $\varphi$ as

$$\varphi(\mathbf{k}) = \arg\left[E_x(\mathbf{k}, z\to\infty) + iE_y(\mathbf{k}, z\to\infty)\right]. \tag{41}$$

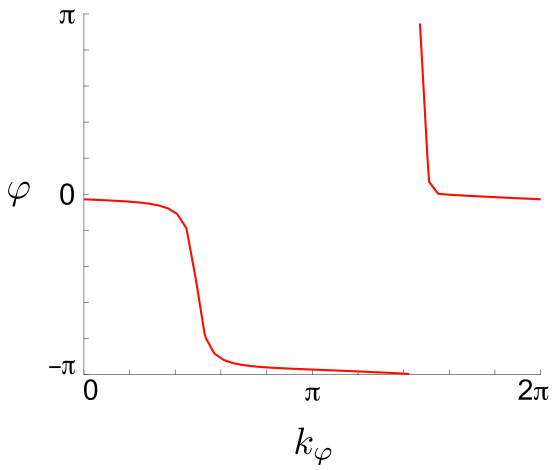


FIG. S9: Evolution of the angle of polarization vector along the closed path in $\mathbf{k}$-space.

We choose a circle with $|\mathbf{k}| = 0.05\pi/p$ and $k_\varphi \in [0, 2\pi]$ as a closed path in $\mathbf{k}$-space, where $p = 1320$ nm is the lattice period. The evolution of $\varphi$ along the path is shown in Fig. S9. The integration in Eq. 40 results in $q_{\rm top} = 1$.

[1] F. Alpeggiani, N. Parappurath, E. Verhagen, and L. Kuipers, Quasinormal-mode expansion of the scattering matrix, Phys. Rev. X **7**, 021035 (2017).
[2] A. B. Evlyukhin, C. Reinhardt, A. Seidel, B. S. Lukyanchuk, and B. N. Chichkov, Optical response features of Si-nanoparticle arrays, Phys. Rev. B **82**, 045404 (2010).
[3] T. Weiss, M. Mesch, M. Schäferling, H. Giessen, W. Langbein, and E. Muljarov, From dark to bright: First-order perturbation theory with analytical mode normalization for plasmonic nanoantenna arrays applied to refractive index sensing, Phys. Rev. Lett. **116**, 237401 (2016).
[4] J. S. T. Gongora, G. Favraud, and A. Fratalocchi, Fundamental and high-order anapoles in all-dielectric metamaterials via Fano-Feshbach modes competition, Nanotechnology **28**, 104001 (2017).
[5] A. B. Evlyukhin, T. Fischer, C. Reinhardt, and B. N. Chichkov, Optical theorem and multipole scattering of light by arbitrarily shaped nanoparticles. Phys. Rev. B **94**, 205434 (2016).
[6] B. Zhen, C.W. Hsu, L. Lu, A.D. Stone, and M. Soljaĉić, Topological nature of optical bound states in the continuum, Phys. Rev. Lett. **113**, 257401 (2014).
